# Supplementary material for: Improving Multimodal Learning with Multi-Loss Gradient Modulation
Source: arXiv:2405.07930 source file (2024-10-14)
Supplement: Supplementary file 1 [file 8-Supplementary.tex]

\clearpage

\setcounter{page}{1}
% \maketitlesupplementary

{
% \newpage 
\twocolumn[
    \centering
    \Large
    \textbf{\thetitle}\\
    \vspace{0.5em}Supplementary Material \\
    \vspace{1.0em}

    % \begin{table*}
    % \renewcommand{\arraystretch}{1.2}
    % \caption{Top-1 accuracy comparison between various models, Ensemble, Late Fusion, Mid-Late Fusion, and Mid Fusion with various balancing techniques that apply to each model. Below the dashed line we can see the models that use unimodally pretrained encoders. In all three datasets, CREMA-D, AVE and UCF101, models using pretrained encoders exceed all previous methods.}
    % \label{table:results}
    % \begin{small}
    % \centering
    % \begin{adjustbox}{scale=0.96} 
    \footnotesize
    
    \captionof{table}{Top-1 accuracy comparison between various models, Ensemble, Late Fusion, Mid-Late Fusion, and Mid Fusion with various balancing techniques that apply to each model. Below the dashed line we can see the models that use unimodally pretrained encoders. In all three datasets, CREMA-D, AVE and UCF101, models using pretrained encoders exceed all previous methods.\label{table:results}}
    \vspace{0.7em}
    \begin{tabular}{ll|lll|lll|lll}
    
            \multicolumn{2}{c}{} & \multicolumn{3}{c}{CREMA-D} & \multicolumn{3}{c}{AVE} & \multicolumn{3}{c}{UCF101}\\
            \cmidrule(lr){3-5}
            \cmidrule(lr){6-8}
            \cmidrule(lr){9-11}
             \multicolumn{2}{c|}{Model: ResNet-18} & MM & Audio & Vision & MM & Audio & Vision & MM & Audio & Vision \\
            \toprule
            & Unimodals &
            & 60.60{\tiny$\pm$2.31} & 55.38{\tiny$\pm$2.97} & %CREMA-D
            & 62.60{\tiny$\pm$0.94} & 45.69{\tiny$\pm$1.63} &  
            & 30.33{\tiny$\pm$1.49} & 38.43{\tiny$\pm$0.96}\\
    
            & Ensemble & 
            71.74{\tiny$\pm$2.08} & 60.60{\tiny$\pm$2.31} & 55.38{\tiny$\pm$2.97} %CREMA-D
            & 70.48{\tiny$\pm$0.23} & 62.60{\tiny$\pm$0.94} & 45.69{\tiny$\pm$1.63}
            & 52.84{\tiny$\pm$0.06} & 30.33{\tiny$\pm$1.49} & 38.43{\tiny$\pm$0.96} \\
            % & Pre Finetuned &  
            % 71.88{\tiny$\pm$2.16} &
            % 55.40{\tiny$\pm$1.49} & 
            % 59.54{\tiny$\pm$0.75} \\
    
            \midrule
    
            \multirow{10}{*}{\rotatebox{90}{Late Fusion}}& 
            Joint Training &  
            61.30{\tiny$\pm$1.36} & 60.05{\tiny$\pm$2.20} & 19.69{\tiny$\pm$0.55} &  %CREMA-D
            67.58{\tiny$\pm$1.02} & 60.12{\tiny$\pm$1.35} & 24.05{\tiny$\pm$1.19} &     
            50.67{\tiny$\pm$2.24} & 28.35{\tiny$\pm$3.33} & 31.37{\tiny$\pm$1.01} \\
            
            % & Modality-Drop \cite{feichtenhofer2019slowfast}   &     
            % -&-&-&
            % -&-&-&
            % -&-&-\\
            
            & MMCosine \cite{xu2023mmcosine}&
            58.83{\tiny$\pm$1.57} & 59.40{\tiny$\pm$1.46} & 20.38{\tiny$\pm$0.51}&     %CREMA-D
            68.99{\tiny$\pm$0.92} & 60.86{\tiny$\pm$1.38} & 25.29{\tiny$\pm$1.50}&
            52.34{\tiny$\pm$3.61} & 24.96{\tiny$\pm$2.20} & 29.01{\tiny$\pm$3.30} \\

            & MSLR \cite{MSLR}&
            56.95{\tiny$\pm$0.00} & 55.51{\tiny$\pm$0.00} & 22.69{\tiny$\pm$0.00}&   %CREMA-D  
            66.75{\tiny$\pm$1.73} & 58.13{\tiny$\pm$1.29} & 25.21{\tiny$\pm$1.02}&
            47.47{\tiny$\pm$3.80} & 24.37{\tiny$\pm$2.22} & 27.77{\tiny$\pm$2.39}\\
    
            & OGM \cite{OGMGE} & 
            {\color{red}{69.30{\tiny$\pm$0.83}} }& {\color{red}{48.98{\tiny$\pm$0.67}} }& {\color{red}{49.43{\tiny$\pm$2.04}}} &
            % 59.94{\tiny$\pm$2.06} & 59.87{\tiny$\pm$1.62} & 19.59{\tiny$\pm$0.83} & %CREMA-D  
            64.93{\tiny$\pm$0.20} & 58.04{\tiny$\pm$0.12} & 27.53{\tiny$\pm$3.55} &
            50.56{\tiny$\pm$2.31} & 23.44{\tiny$\pm$1.39} & 31.72{\tiny$\pm$2.58}\\
    
            & OGMGE \cite{OGMGE} & 
            58.39{\tiny$\pm$1.35} & 58.55{\tiny$\pm$0.44} & 20.68{\tiny$\pm$0.66} & %CREMA-D  
            66.42{\tiny$\pm$0.41} & 60.28{\tiny$\pm$0.94} & 22.97{\tiny$\pm$0.92} &
            49.33{\tiny$\pm$3.15} & 28.07{\tiny$\pm$2.87} & 31.35{\tiny$\pm$0.95}\\

            & AGM \cite{AGM} & 
             71.42{\tiny$\pm$2.30} & 55.88{\tiny$\pm$0.94} & 50.73{\tiny$\pm$3.36} &     %CREMA-D  
            64.43{\tiny$\pm$1.42} & 55.56{\tiny$\pm$1.38} & 29.44{\tiny$\pm$2.93} &
            48.12{\tiny$\pm$4.06} & 25.97{\tiny$\pm$2.76} & 31.91{\tiny$\pm$2.47}\\
            
            & PMR \cite{PMR}&
            53.63{\tiny$\pm$1.37} & 52.94{\tiny$\pm$1.15} & 20.78{\tiny$\pm$0.39}&
            37.40{\tiny$\pm$7.55} & 16.00{\tiny$\pm$16.30} & 25.95{\tiny$\pm$5.84}&
            40.86{\tiny$\pm$2.01} & 19.02{\tiny$\pm$2.51} & 28.86{\tiny$\pm$1.67} \\
            
            & Multi-Loss&
            69.18{\tiny$\pm$1.64} & 54.07{\tiny$\pm$0.66} & 54.85{\tiny$\pm$1.48} & 
            70.56{\tiny$\pm$0.23} & 61.53{\tiny$\pm$0.51} & 39.64{\tiny$\pm$3.93} & 
            52.58{\tiny$\pm$1.81} & 29.33{\tiny$\pm$2.35} & 40.43{\tiny$\pm$1.16}\\
                   
            \cdashline{2-11}
    
            &Pre Enc Frozen &   
            73.46{\tiny$\pm$2.71} & 59.18{\tiny$\pm$1.80} & 55.82{\tiny$\pm$3.06} &
            72.14{\tiny$\pm$0.20} & 61.44{\tiny$\pm$1.06} & 45.94{\tiny$\pm$0.92} &
            53.40{\tiny$\pm$1.29} & 30.58{\tiny$\pm$1.42} & 37.64{\tiny$\pm$1.00} \\
             
            &Pre Enc Finetuned  &    
            73.33{\tiny$\pm$1.40} & 59.91{\tiny$\pm$2.28} & 55.38{\tiny$\pm$1.54} &
            72.39{\tiny$\pm$0.54} & 61.94{\tiny$\pm$0.73} & 43.70{\tiny$\pm$0.62} &
            53.35{\tiny$\pm$1.60} & 30.54{\tiny$\pm$1.54} & 35.45{\tiny$\pm$0.92}\\

            \midrule
    
            \multirow{7}{*}{\rotatebox{90}{Mid Late Fusion}}& Joint Training & 
            56.41{\tiny$\pm$2.69} & 57.42{\tiny$\pm$0.95} & 20.42{\tiny$\pm$0.52} & %H
             63.43{\tiny$\pm$0.73} & 57.38{\tiny$\pm$2.35} & 21.64{\tiny$\pm$1.33} &
            39.02{\tiny$\pm$5.35} & 24.54{\tiny$\pm$2.57} & 28.34{\tiny$\pm$1.29} \\

            & MMCosine \cite{xu2023mmcosine}&
             57.54{\tiny$\pm$2.00} & 57.68{\tiny$\pm$1.36} & 19.69{\tiny$\pm$0.63}&
            62.69{\tiny$\pm$2.54} & 57.88{\tiny$\pm$1.92} & 23.55{\tiny$\pm$1.31}&
            41.66{\tiny$\pm$3.32} & 24.59{\tiny$\pm$2.13} & 29.23{\tiny$\pm$1.85}\\
            
            & AGM \cite{AGM} & 
            70.36{\tiny$\pm$1.77} & 54.95{\tiny$\pm$2.81} & 50.66{\tiny$\pm$0.53} &
            64.18{\tiny$\pm$1.27} & 48.59{\tiny$\pm$15.38} & 22.89{\tiny$\pm$7.30}&
            45.75{\tiny$\pm$3.40} & 24.12{\tiny$\pm$2.18} & 32.98{\tiny$\pm$3.79}\\
            
            & Multi-Loss &
            65.39{\tiny$\pm$5.73} & 54.47{\tiny$\pm$2.47} & 43.78{\tiny$\pm$16.74}&
            65.84{\tiny$\pm$0.82} & 56.55{\tiny$\pm$1.44} & 46.77{\tiny$\pm$0.20}&
            44.88{\tiny$\pm$3.25} & 25.30{\tiny$\pm$3.77} & 34.87{\tiny$\pm$4.86}\\
            
            \cdashline{2-11}
    
            &Pre Enc Frozen& 
             72.00{\tiny$\pm$1.46} & 56.67{\tiny$\pm$2.08} & 54.83{\tiny$\pm$2.63} & %H
            69.32{\tiny$\pm$1.00} & 61.19{\tiny$\pm$1.77} & 46.10{\tiny$\pm$1.77}&
             44.95{\tiny$\pm$1.29} & 30.75{\tiny$\pm$1.27} & 38.14{\tiny$\pm$2.00} \\
    
            &Pre Enc Finetuned & 
            71.21{\tiny$\pm$3.18} & 51.51{\tiny$\pm$1.81} & 47.12{\tiny$\pm$2.60} & %H
            70.98{\tiny$\pm$0.51} & 60.70{\tiny$\pm$1.46} & 45.94{\tiny$\pm$1.52}&
            47.38{\tiny$\pm$2.30} & 29.73{\tiny$\pm$1.55} & 38.57{\tiny$\pm$2.04}\\
    
            \midrule
    
            \multirow{7}{*}{\rotatebox{90}{Mid Fusion}}& Joint Training & 
            55.60{\tiny$\pm$1.14} & 56.47{\tiny$\pm$0.85} & 20.56{\tiny$\pm$0.28} & %H
            62.77{\tiny$\pm$1.89} & 51.49{\tiny$\pm$3.39} & 7.05{\tiny$\pm$2.07} &
            39.53{\tiny$\pm$1.18} & 26.44{\tiny$\pm$2.84} & 27.88{\tiny$\pm$2.27}\\

            & MMCosine \cite{xu2023mmcosine}&
            55.10{\tiny$\pm$2.68} & 55.36{\tiny$\pm$1.89} & 20.74{\tiny$\pm$0.06}&
            59.95*{\tiny$\pm$1.24} & 54.48{\tiny$\pm$0.50} & 20.15{\tiny$\pm$0.25}&
            39.48{\tiny$\pm$3.91} & 23.81{\tiny$\pm$1.59} & 29.20{\tiny$\pm$1.13}\\
            
            & AGM \cite{AGM} & 
            63.13{\tiny$\pm$11.92} & 42.66{\tiny$\pm$20.17} & 38.84{\tiny$\pm$15.22} &
            64.10{\tiny$\pm$1.24} & 57.13{\tiny$\pm$1.24} & 29.52{\tiny$\pm$2.00}&
            42.68{\tiny$\pm$2.82} & 23.87{\tiny$\pm$2.65} & 31.24{\tiny$\pm$0.24}\\
            
            & Multi-Loss &
            55.14{\tiny$\pm$2.11} & 55.10{\tiny$\pm$2.31} & 20.78{\tiny$\pm$0.39}&
             66.17{\tiny$\pm$2.00} & 53.90{\tiny$\pm$1.64} & 43.12{\tiny$\pm$4.46}&
            48.51{\tiny$\pm$3.79} & 25.63{\tiny$\pm$1.93} & 40.82{\tiny$\pm$2.26}\\
            
            \cdashline{2-11}
    
            &Pre Enc Frozen& 
             69.08{\tiny$\pm$3.33} & 59.58{\tiny$\pm$1.83} & 55.85{\tiny$\pm$3.13} & %H
            70.32{\tiny$\pm$0.31} & 59.45{\tiny$\pm$0.89} & 36.73{\tiny$\pm$1.43}&
            44.56{\tiny$\pm$2.05} & 30.90{\tiny$\pm$1.20} & 38.03{\tiny$\pm$2.18}\\
            
            &Pre Enc Finetuned & 
             70.40{\tiny$\pm$2.57} & 59.38{\tiny$\pm$1.09} & 55.89{\tiny$\pm$2.98}  & %H
            69.73{\tiny$\pm$0.31} & 60.53{\tiny$\pm$1.12} & 43.03{\tiny$\pm$0.54}&
            46.12{\tiny$\pm$1.17} & 30.25{\tiny$\pm$1.07} & 39.20{\tiny$\pm$2.37}\\
    
            \bottomrule
        \end{tabular} 
    \vspace{1.5em}
   ] %< twocolumn
}

{
% \newpage 
\twocolumn[
    \centering
    \Large
    \textbf{\thetitle}\\
    \vspace{0.5em}Supplementary Material \\
    \vspace{1.0em}

    % \begin{table*}
    % \renewcommand{\arraystretch}{1.2}
    % \caption{Top-1 accuracy comparison between various models, Ensemble, Late Fusion, Mid-Late Fusion, and Mid Fusion with various balancing techniques that apply to each model. Below the dashed line we can see the models that use unimodally pretrained encoders. In all three datasets, CREMA-D, AVE and UCF101, models using pretrained encoders exceed all previous methods.}
    % \label{table:results}
    % \begin{small}
    % \centering
    % \begin{adjustbox}{scale=0.96} 
    \footnotesize
    
    \captionof{table}{Top-1 accuracy comparison between various models, Ensemble, Late Fusion, Mid-Late Fusion, and Mid Fusion with various balancing techniques that apply to each model. Below the dashed line we can see the models that use unimodally pretrained encoders. In all three datasets, CREMA-D, AVE and UCF101, models using pretrained encoders exceed all previous methods.\label{table:results}}
    \vspace{0.7em}
    \begin{tabular}{ll|lll|lll|lll}
    
            \multicolumn{2}{c}{} & \multicolumn{3}{c}{CREMA-D} & \multicolumn{3}{c}{AVE} & \multicolumn{3}{c}{UCF101}\\
            \cmidrule(lr){3-5}
            \cmidrule(lr){6-8}
            \cmidrule(lr){9-11}
             \multicolumn{2}{c|}{Model: Wav2Vec+Conformer} & MM & Audio & Vision & MM & Audio & Vision & MM & Audio & Vision \\
            \toprule
            & Unimodals &
            & 76.75{\tiny$\pm$2.72} & 69.42{\tiny$\pm$1.96} & %CREMA-D
            -{\tiny$\pm$-} & -{\tiny$\pm$-} & -{\tiny$\pm$-}& 
            -{\tiny$\pm$-} & -{\tiny$\pm$-} & -{\tiny$\pm$-} \\
    
            & Ensemble & 
            83.94{\tiny$\pm$3.05} & 76.75{\tiny$\pm$2.72} & 69.42{\tiny$\pm$1.96} %CREMA-D
            & 
            -{\tiny$\pm$-} & -{\tiny$\pm$-} & -{\tiny$\pm$-}& 
            -{\tiny$\pm$-} & -{\tiny$\pm$-} & -{\tiny$\pm$-} \\
            % & Pre Finetuned &  
            % 71.88{\tiny$\pm$2.16} &
            % 55.40{\tiny$\pm$1.49} & 
            % 59.54{\tiny$\pm$0.75} \\
    
            \midrule
    
            \multirow{10}{*}{\rotatebox{90}{Late Fusion}}& 
            Joint Training &  
            74.09{\tiny$\pm$4.38} & 47.72{\tiny$\pm$7.07} & 67.31{\tiny$\pm$1.51} & 
            -{\tiny$\pm$-} & -{\tiny$\pm$-} & -{\tiny$\pm$-}& 
            -{\tiny$\pm$-} & -{\tiny$\pm$-} & -{\tiny$\pm$-} \\

            & MMCosine \cite{xu2023mmcosine}&
            -{\tiny$\pm$-} & -{\tiny$\pm$-} & -{\tiny$\pm$-}& 
            -{\tiny$\pm$-} & -{\tiny$\pm$-} & -{\tiny$\pm$-}& 
            -{\tiny$\pm$-} & -{\tiny$\pm$-} & -{\tiny$\pm$-} \\

            & MSLR \cite{MSLR}&
            -{\tiny$\pm$-} & -{\tiny$\pm$-} & -{\tiny$\pm$-}& 
            -{\tiny$\pm$-} & -{\tiny$\pm$-} & -{\tiny$\pm$-}& 
            -{\tiny$\pm$-} & -{\tiny$\pm$-} & -{\tiny$\pm$-} \\
    
            & OGM \cite{OGMGE} & 
            -{\tiny$\pm$-} & -{\tiny$\pm$-} & -{\tiny$\pm$-}& 
            -{\tiny$\pm$-} & -{\tiny$\pm$-} & -{\tiny$\pm$-}& 
            -{\tiny$\pm$-} & -{\tiny$\pm$-} & -{\tiny$\pm$-} \\
    
            & OGMGE \cite{OGMGE} & 
            -{\tiny$\pm$-} & -{\tiny$\pm$-} & -{\tiny$\pm$-}& 
            -{\tiny$\pm$-} & -{\tiny$\pm$-} & -{\tiny$\pm$-}& 
            -{\tiny$\pm$-} & -{\tiny$\pm$-} & -{\tiny$\pm$-} \\

            & AGM \cite{AGM} & 
            -{\tiny$\pm$-} & -{\tiny$\pm$-} & -{\tiny$\pm$-}& 
            -{\tiny$\pm$-} & -{\tiny$\pm$-} & -{\tiny$\pm$-}& 
            -{\tiny$\pm$-} & -{\tiny$\pm$-} & -{\tiny$\pm$-} \\
            
            & PMR \cite{PMR}&
            -{\tiny$\pm$-} & -{\tiny$\pm$-} & -{\tiny$\pm$-}& 
            -{\tiny$\pm$-} & -{\tiny$\pm$-} & -{\tiny$\pm$-}& 
            -{\tiny$\pm$-} & -{\tiny$\pm$-} & -{\tiny$\pm$-} \\

            & Multi-Loss&
         83.80{\tiny$\pm$1.46} & 77.05{\tiny$\pm$1.73} & 68.45{\tiny$\pm$1.37}& 
            -{\tiny$\pm$-} & -{\tiny$\pm$-} & -{\tiny$\pm$-}& 
            -{\tiny$\pm$-} & -{\tiny$\pm$-} & -{\tiny$\pm$-} \\

            \cdashline{2-11}
    
            &Pre Enc Frozen &   
            84.93{\tiny$\pm$3.11} & 76.91{\tiny$\pm$1.75} & 
            69.16{\tiny$\pm$1.55}& 
            -{\tiny$\pm$-} & -{\tiny$\pm$-} & -{\tiny$\pm$-}& 
            -{\tiny$\pm$-} & -{\tiny$\pm$-} & -{\tiny$\pm$-} \\
             
            &Pre Enc Finetuned  &    
            -{\tiny$\pm$-} & -{\tiny$\pm$-} & -{\tiny$\pm$-}& 
            -{\tiny$\pm$-} & -{\tiny$\pm$-} & -{\tiny$\pm$-}& 
            -{\tiny$\pm$-} & -{\tiny$\pm$-} & -{\tiny$\pm$-} \\

            \midrule
    
            \multirow{7}{*}{\rotatebox{90}{Mid Late Fusion}}& Joint Training & 
            -{\tiny$\pm$-} & -{\tiny$\pm$-} & -{\tiny$\pm$-}& 
            -{\tiny$\pm$-} & -{\tiny$\pm$-} & -{\tiny$\pm$-}& 
            -{\tiny$\pm$-} & -{\tiny$\pm$-} & -{\tiny$\pm$-} \\

            & MMCosine \cite{xu2023mmcosine}&
            -{\tiny$\pm$-} & -{\tiny$\pm$-} & -{\tiny$\pm$-}& 
            -{\tiny$\pm$-} & -{\tiny$\pm$-} & -{\tiny$\pm$-}& 
            -{\tiny$\pm$-} & -{\tiny$\pm$-} & -{\tiny$\pm$-} \\
            
            & AGM \cite{AGM} & 
             -{\tiny$\pm$-} & -{\tiny$\pm$-} & -{\tiny$\pm$-}& 
            -{\tiny$\pm$-} & -{\tiny$\pm$-} & -{\tiny$\pm$-}& 
            -{\tiny$\pm$-} & -{\tiny$\pm$-} & -{\tiny$\pm$-} \\
            
            & Multi-Loss &
            -{\tiny$\pm$-} & -{\tiny$\pm$-} & -{\tiny$\pm$-}& 
            -{\tiny$\pm$-} & -{\tiny$\pm$-} & -{\tiny$\pm$-}& 
            -{\tiny$\pm$-} & -{\tiny$\pm$-} & -{\tiny$\pm$-} \\
            
            \cdashline{2-11}
    
            &Pre Enc Frozen& 
            -{\tiny$\pm$-} & -{\tiny$\pm$-} & -{\tiny$\pm$-}& 
            -{\tiny$\pm$-} & -{\tiny$\pm$-} & -{\tiny$\pm$-}& 
            -{\tiny$\pm$-} & -{\tiny$\pm$-} & -{\tiny$\pm$-} \\
    
            &Pre Enc Finetuned & 
            -{\tiny$\pm$-} & -{\tiny$\pm$-} & -{\tiny$\pm$-}& 
            -{\tiny$\pm$-} & -{\tiny$\pm$-} & -{\tiny$\pm$-}& 
            -{\tiny$\pm$-} & -{\tiny$\pm$-} & -{\tiny$\pm$-} \\
    
            \midrule
    
            \multirow{7}{*}{\rotatebox{90}{Mid Fusion}}& Joint Training & 
            -{\tiny$\pm$-} & -{\tiny$\pm$-} & -{\tiny$\pm$-}& 
            -{\tiny$\pm$-} & -{\tiny$\pm$-} & -{\tiny$\pm$-}& 
            -{\tiny$\pm$-} & -{\tiny$\pm$-} & -{\tiny$\pm$-} \\

            & MMCosine \cite{xu2023mmcosine}&
            -{\tiny$\pm$-} & -{\tiny$\pm$-} & -{\tiny$\pm$-}& 
            -{\tiny$\pm$-} & -{\tiny$\pm$-} & -{\tiny$\pm$-}& 
            -{\tiny$\pm$-} & -{\tiny$\pm$-} & -{\tiny$\pm$-} \\
            
            & AGM \cite{AGM} & 
            -{\tiny$\pm$-} & -{\tiny$\pm$-} & -{\tiny$\pm$-}& 
            -{\tiny$\pm$-} & -{\tiny$\pm$-} & -{\tiny$\pm$-}& 
            -{\tiny$\pm$-} & -{\tiny$\pm$-} & -{\tiny$\pm$-} \\
            
            & Multi-Loss &
            -{\tiny$\pm$-} & -{\tiny$\pm$-} & -{\tiny$\pm$-}& 
            -{\tiny$\pm$-} & -{\tiny$\pm$-} & -{\tiny$\pm$-}& 
            -{\tiny$\pm$-} & -{\tiny$\pm$-} & -{\tiny$\pm$-} \\
            
            \cdashline{2-11}
    
            &Pre Enc Frozen& 
            -{\tiny$\pm$-} & -{\tiny$\pm$-} & -{\tiny$\pm$-}& 
            -{\tiny$\pm$-} & -{\tiny$\pm$-} & -{\tiny$\pm$-}& 
            -{\tiny$\pm$-} & -{\tiny$\pm$-} & -{\tiny$\pm$-} \\
            
            &Pre Enc Finetuned & 
            -{\tiny$\pm$-} & -{\tiny$\pm$-} & -{\tiny$\pm$-}& 
            -{\tiny$\pm$-} & -{\tiny$\pm$-} & -{\tiny$\pm$-}& 
            -{\tiny$\pm$-} & -{\tiny$\pm$-} & -{\tiny$\pm$-} \\
    
            \bottomrule
        \end{tabular} 
    \vspace{1.5em}
   ] %< twocolumn
}
% \twocolumn[
% \begin{table}[!htbp]
% \renewcommand{\arraystretch}{1.2}
% \caption{Top-1 accuracy comparison between various models, Ensemble, Late Fusion, Mid-Late Fusion, and Mid Fusion with various balancing techniques that apply to each model. Below the dashed line we can see the models that use unimodally pretrained encoders. In all three datasets, CREMA-D, AVE and UCF101, models using pretrained encoders exceed all previous methods.}
% \label{table:results}
% \begin{small}
% \centering
% \begin{adjustbox}{scale=0.96} 
% \end{adjustbox}
% \end{small}
% \end{table}
% ]

\appendix

\section{Appendix}

\subsection{Test-Validation Sets}

It is important to note that the methods introduced in \cite{AGM, OGMGE, xu2023mmcosine, PMR}, and based on the code they shared, employed the test set as the validation set, tuning model parameters directly on the test set. Therefore, the observed performance difference in our results compared to the initially reported results is attributed to the fact that we validate the models with a separate validation set, comprising around 10\% of the total data. Additionally, in CREMA-D, prior works have included the same actors in different sets, rewarding models that overfit.

\subsection{Table Results}

In Table \ref{table:results}, we present our results in a tabular format for improved clarity and reproducibility, adopting a structure commonly used in prior work. The table includes various models categorized by fusion method—Late Fusion, Mid-Late Fusion, and Mid Fusion—across three distinct datasets: CREMA-D, AVE, and UCF101. The top rows display unimodal trained models and the Ensemble, while the rows below the dashed line in each fusion method section showcase models utilizing pretrained unimodal encoders. Each column section reports the performance of unimodal and multimodal models. This table facilitates for a straightforward comparison of the absolute differences among the models and their baselines.

\subsection{EXTRA: Results on Sth-Sth with Swin-T and STLT}

{
% \newpage 
\twocolumn[
    \centering
    \Large
    \textbf{\thetitle}\\
    \vspace{0.5em}Supplementary Material \\
    \vspace{1.0em}

    % \begin{table*}
    % \renewcommand{\arraystretch}{1.2}
    % \caption{Top-1 accuracy comparison between various models, Ensemble, Late Fusion, Mid-Late Fusion, and Mid Fusion with various balancing techniques that apply to each model. Below the dashed line we can see the models that use unimodally pretrained encoders. In all three datasets, CREMA-D, AVE and UCF101, models using pretrained encoders exceed all previous methods.}
    % \label{table:results}
    % \begin{small}
    % \centering
    % \begin{adjustbox}{scale=0.96} 
    \footnotesize
    
    \captionof{table}{Top-1 accuracy comparison between various models, Ensemble, Late Fusion, Mid-Late Fusion, and Mid Fusion with various balancing techniques that apply to each model. Below the dashed line we can see the models that use unimodally pretrained encoders. In all three datasets, CREMA-D, AVE and UCF101, models using pretrained encoders exceed all previous methods.\label{table:results}}
    \vspace{0.7em}
    \begin{tabular}{ll|llll}
    
            \multicolumn{2}{c}{} & \multicolumn{4}{c}{Something-Something (Top1/Top5 Accuracy)}\\
            \cmidrule(lr){3-6}
             \multicolumn{2}{c|}{Model: Swin-T \& STLT} & MM & Video & Flow & OBJ  \\
            \toprule
            % & Unimodals &
            % & 59.86/86.44 & 38.43{\tiny$\pm$0.96} & \\
    
            % & Ensemble & 51.68/81.02
            % & 59.86/86.44 & 30.33{\tiny$\pm$1.49} & 38.43{\tiny$\pm$0.96} & \\

            & Unimodals &
            & 61.26/87.12  & 50.63/80.35 & 47.51/75.89\\

            & Ensemble & 66.70/90.74 & 61.26/87.12  & 50.63/80.35 & 47.51/75.89\\
            \midrule
            
            & Joint Training & 58.76/85.02 & 55.95/82.91 & 1.21/6.60  \\
            % & AGM \cite{AGM} &  - & - & -\\
            & Multi-Loss  &  59.72/- & 52.94 & 45.83/-& 1.21/-\\
            \cdashline{2-6}
    
            &Pre Enc Frozen  &  67.22/90.94 & 61.26/87.12  & 50.63/80.35 & 47.51/75.89 \\

            &Pre Enc  & 67.05/90.68 & -/- & -/- & -/- \\
   
            \bottomrule
        \end{tabular} 
    \vspace{1.5em}
   ] %< twocolumn
}

{
% \newpage 
\twocolumn[
    \centering
    \Large
    \textbf{\thetitle}\\
    \vspace{0.5em}Supplementary Material \\
    \vspace{1.0em}

    % \begin{table*}
    % \renewcommand{\arraystretch}{1.2}
    % \caption{Top-1 accuracy comparison between various models, Ensemble, Late Fusion, Mid-Late Fusion, and Mid Fusion with various balancing techniques that apply to each model. Below the dashed line we can see the models that use unimodally pretrained encoders. In all three datasets, CREMA-D, AVE and UCF101, models using pretrained encoders exceed all previous methods.}
    % \label{table:results}
    % \begin{small}
    % \centering
    % \begin{adjustbox}{scale=0.96} 
    \footnotesize
    
    \captionof{table}{}
    \vspace{0.7em}
    \begin{tabular}{ll|llll}
    
            \multicolumn{2}{c}{} & \multicolumn{4}{c}{CMU MOSEI (Top2/Top7 Accuracy)}\\
            \cmidrule(lr){3-6}
             \multicolumn{2}{c|}{Model: TF} & MM & Audio & Video & Text  \\
            \toprule
            % & Unimodals &
            % & 59.86/86.44 & 38.43{\tiny$\pm$0.96} & \\
    
            % & Ensemble & 51.68/81.02
            % & 59.86/86.44 & 30.33{\tiny$\pm$1.49} & 38.43{\tiny$\pm$0.96} & \\

            & Unimodals &
            & 64.91/40.97{\tiny$\pm$0.4/0.43}  &65.31/42.19{\tiny$\pm$0.49/0.25} & 78.97/48.83{\tiny$\pm$0.92/0.17}\\
  
            & Ensemble & 77.34/37.43{\tiny$\pm$0.53/1.83} & 64.91/40.97{\tiny$\pm$0.4/0.43}  &65.31/42.19{\tiny$\pm$0.49/0.25} & 78.97/48.83{\tiny$\pm$0.92/0.17}\\
            \midrule
            
            & Joint Training & 80.11/48.5{\tiny$\pm$0.67/0.73} & -/-{\tiny$\pm$-/-}  &-/-{\tiny$\pm$-/-} & -/-{\tiny$\pm$-/-}\\
            % & AGM \cite{AGM} &  - & - & -\\
            & Multi-Loss  & 80.37/49.20{\tiny$\pm$0.67/0.7} & 64.21/41.31{\tiny$\pm$0.28/0.21}  &65.31/41.73{\tiny$\pm$1.05/0.37} & 79.85/48.96{\tiny$\pm$0.33/0.64}\\
            \cdashline{2-6}

            &Pre Enc Frozen  & 80.45/48.96{\tiny$\pm$0.34/0.55} & 46.45/-{\tiny$\pm$-/-}&
            41.13/-{\tiny$\pm$-/-} & 60.4/-{\tiny$\pm$-/-}\\
            
            &Pre Enc  & 80.63/49.06{\tiny$\pm$0.35/0.19} & -/-{\tiny$\pm$-/-}  &-/-{\tiny$\pm$-/-} & -/-{\tiny$\pm$-/-}\\
   
            \bottomrule
        \end{tabular} 
    \vspace{1.5em}
   ] %< twocolumn
}
